# Supplementary material for: Time and Parallelizability Results for Parity Games with Bounded Tree and DAG Width
Source: arXiv:1112.0221 source file (2013-06-17)
Supplement: Supplementary file 1 [file appendix.tex]

\newpage
\appendix

\section{Preliminaries for
Lemmas~\ref{lem:verifyparity},~\ref{lem:evenwinspace},
and~\ref{lem:oddwinspace}}
\label{sec:prelim}

In this section we will give notation and auxiliary lemmas that will be used in
later proofs. Although the two games $\verify$ and $\spaceverify$ have different
winning conditions, the way that the players construct the path $\Pi$ is the
same in both games. In this section we describe how, if certain conditions are
met, the paths~$\Pi$ must correspond to some path in the parity game, and we
give notation that will allow us to use these paths in the subsequent proofs.

We begin with a simple Lemma that shows that the game $\verify$ cannot go on
forever. We do not need an analogous lemma for $\spaceverify^c$, because this
game is guaranteed to end after $c$ rounds have been played.

\section{Proof of Theorem~\ref{thm:time}}

%\section{Proof of Lemma~\ref{lem:winspace}}

%In this proof, we reuse the strategies $\win(\sigma)$ for $\sigma \in \Sigma_0$,
%and $\win(\tau)$ for $\tau \in \Sigma_1$, which were defined
%Appendix~\ref{sec:verifyparity} for the proof of Lemma~\ref{lem:verifyparity}.
%Note that, if we ignore the choice of $S'$ that Odd must make, these strategies
%are still well defined in $\spaceverify$. This lemma has two cases, which will
%be proved separately. First we consider the case where $s \in W_0$.

%%%%%%%%%%%%%%%%%% CUT POINT %%%%%%%%%%%%%%%%%%%%%%%%%%%%%%%%%%

%We now move on to prove the case where Odd has a winning strategy $\tau$ for a
%vertex $s \in W_1$. In this proof we ignore the fact that Odd must choose a set
%$S'$, by assuming that an arbitrary set is chosen whenever a decision must be
%made by Odd. The purpose of this proof is to show that, no matter what sets are
%chosen, if the game terminates before round $r+1$, then $\win(\tau)$ will ensure
%that Odd wins the game.

%%%%%%%%%%%%%%%%%% CUT POINT %%%%%%%%%%%%%%%%%%%%%%%%%%%%%%%%%%

\section{Proof of Lemma~\ref{lem:oddchooseset}}

\section{Proof of Theorem~\ref{thm:space}}
